# Supplementary material for: Graph-based Diffusion Model for Collaborative Filtering
Source: arXiv:2504.05029 source file (2025-04-07)
Supplement: Supplementary file 1 [file appendix.tex]

% \FloatBarrier
% \begin{table*}[]
% \centering
% \begin{tabular}{|c|l|}
% \hline
% \hline
% \textbf{Symbol} & \textbf{Description} \\ \hline
% $\mathcal{G} = (\mathcal{V}, \mathcal{E})$    & bipartite graph where $\mathbf{X} \in  \mathbb{R}^{(M+N) \times d_x}$ is the matrix of node features and $\mathbf{R}$ is the interaction matrix, $r_{ui}$ is the element of $\mathbf{R}$  \\ \hline
% $\mathcal{U}$ & the user set in recommendation system \\\hline
% $\mathcal{I}$ & the item set in recommendation system\\ \hline
% $M$ & the number of user in recommendation system \\\hline
% $N$ & the number of item in recommendation system \\\hline
% $u$             & a user node in the bipartite graph \\ \hline
% $i$             & an item node in the bipartite graph \\ \hline
% $A_{\mathcal{G}}$             & the adjacency matrix of $\mathcal{G}$ \\ \hline
% $D_{\mathcal{G}}$             & the degree matrix of $\mathcal{G}$ \\ \hline
% $\mathbf{y}$             & data sample \\ \hline
% $\mathbf{z}$             & noise point \\ \hline
% $t$             & diffusion step \\ \hline
% $\phi_{\theta}$             & denoising model \\ \hline
% $L$             & the number of GCNs layers\\ \hline
% $Z^{(l)}$             & aggregated representations from the l-th layer of GCNs, $z^{(l)}_u$ is the representation of user $u$ of $l$-th layer at vector level   \\ \hline
% $F$             & aggregation function \\ \hline
% $f_c$             & combination function at vector level \\ \hline
% $f_{agg}$             & aggregation function at vector level\\ \hline
% $f_{o}$             & output function at vector level\\ \hline
% $\mathcal{N}_u$          & Neighborhood of user $u$, i.e., the set of items connected to $u$ \\ \hline
% $\mathcal{N}_i$ & neighbors of item $i$ \\ \hline
% $\mathbf{E}$ & The set of one-hot encodings $e$ for each edge\\ \hline
% $\mathbf{Q}^t$ & the transition probability matrices\\ \hline
% $\beta$ &  the scale of the Gaussian noise  \\ \hline
% $\mathcal{N}$ & Gaussian distribution  \\ \hline
% $\mathcal{G}^t_X$ & continuous corrupted bipartite graph  \\ \hline
% $\mathcal{G}^t_E$ & discrete corrupted bipartite graph \\ \hline
% $X^{\prime}$ & node representation matrix of continuous corrupted bipartite graph   \\ \hline
% $X^{\prime \prime}$ & node representation matrix of discrete corrupted bipartite graph \\ \hline
% \(s(\cdot)\) & the similarity between two representations \\ \hline
% $\boldsymbol{\epsilon}$ & Gaussian-distributed noise \\ \hline
% \(\tau\) & the temperature hyperparameter of the Softmax function \\ \hline
% $\mathcal{L}_{aur}$             & Loss function of alignment module \\ \hline
% \( \mathcal{G}^T \) & the unified corrupted bipartite graph with node feature matrix \( \bar{\mathbf{X}}^T \) and edge matrix \( \bar{\mathbf{E}}^T \)\\ \hline
% $\hat{\mathcal{G}}^0$ & the predicted graph \\ \hline
% $Z_t$ & the node representation matrix after multiple layers of graph convolution \\ \hline
% $\sigma(\cdot)$ & Activation function (e.g., ReLU or sigmoid) \\ \hline
% $\epsilon$      & Noise added during the corruption process \\ \hline
% $t$             & Time step in the forward/reverse process \\ \hline
% \end{tabular}
% \caption{List of symbols used in the paper}
% \end{table*}
